# Supplementary material for: Articulate That Object Part (ATOP): 3D Part Articulation via Text and Motion Personalization
Source: arXiv:2502.07278 source file (2026-05-22)
Supplement: Supplementary file 1 [file supplementary.tex]

\section{Implementation details} Our implementation is based on the Pytorch framework \cite{paszke2019pytorch}. For diffusion, we use a popular library diffusers \cite{von-platen-etal-2022-diffusers}. In both stages i.e. during finetuning as well as during 3D motion transfer stage we use Adam optimizer \cite{kingma2014adam} to update the trainable parameters. During the finetuning stage, we set a learning rate of $5e^{-4}$, whereas during the 3D motion transfer stage, we set a learning rate of $5e^{-3}$. During finetuning, we train the model for $20000$ iterations. A single multi-view video sample comprises of $4$ views and $10$ frames each. The resolution of each video is $256\times256$. During the personalization step, we do inference for $50$ steps using a classifier-free guidance scale of $5.0$. Both finetuning and inference are done with \texttt{fp16} model weights of ImageDream. During inference, we render the image using Blender, whereas the masks are rendered using Pytorch3D \cite{ravi2020accelerating}. We finetune a single personalized diffusion model on Nvidia $V100$ GPU with $32$Gb GPU memory. The training takes approximately 5hrs to complete. During inference, we sample $2048$ points each on both static and dynamic part of the mesh and then initialize the gaussian centers with it. For our renderer, we set $\beta_{1}=21.4$, $\beta_{2}=2.66$. Because we optimize the points within the latent space of the diffusion model, we render features of resolution $32\times32$. 

\section{Algorithm} Here, we explain in detail the algorithm used to retrieve the motion axis and origin from the point cloud. In this paper, we consider two types of motion, 1) Revolute Motion 2) Prismatic Motion. 
\\
\emph{Revolute Motion.} Given a set of vertices of a mesh  $\mathcal{M}$ the revolute motion is represented as: 
\begin{equation}
    \Vec{x}^{*} = \mathbf{R} \ (\Vec{x} - \Vec{o}) + \Vec{o}
    \label{eq: revolute_motion}
\end{equation}
where, $\Vec{x}$ is the original mesh vertex, $\Vec{x}^{*}$ is the transformed mesh vertex after articulation, $\Vec{o}$ is motion axis origin, $\mathbf{R}$ is the rotation matrix around the predicted motion axis direction, $\Vec{a}=[a_{x},\ a_{y},\ a_{z}]$. Here, $\|\Vec{a}\|=1$. Given an angle $\theta$, with which we want to rotate around the motion axis, we can compute the rotation matrix using Rodrigues formula as,
\begin{gather}
\mathbf{K} =
\begin{bmatrix}
0 & -\text{a}_z & \text{a}_y \\
\text{a}_z & 0 & -\text{a}_x \\
-\text{a}_y & \text{a}_x & 0
\end{bmatrix}, \\
\mathbf{R} = \mathbf{I} + \sin(\theta) \ \mathbf{K} + (1 - \cos(\theta)) \ \mathbf{K}^2
\end{gather}
\emph{Prismatic Motion.} Unlike revolute motion, prismatic motion is defined using only motion axis, $\Vec{a}$, where $\|\Vec{a}\|=1$. Given a motion range $[M_{max}, M_{min}]$ within which we would like to articulate a part, the magnitude $\gamma$ and ultimately the transformed vertex of the mesh $\mathcal{M}$ is defined as:
\begin{equation}
    \Vec{a}^{*} = \gamma * \Vec{a}, \quad \Vec{x}^{*} = \Vec{x} + \Vec{a}^{*}
    \label{eq: prismatic_motion}
\end{equation}
where, $\gamma$ is the magnitude of scaling computed from the motion range, $\Vec{x}$ is the original mesh vertex and $\Vec{x}^{*}$ is the transformed mesh vertex. The algorithm to find motion parameters is described in Algorithm \ref{alg:find_motion_parameters}.

\begin{algorithm}
    \SetCommentSty{commfont}
    \SetKwInOut{Input}{input}\SetKwInOut{Output}{output}
    \Input{Static Mesh $\mathcal{M}$, Point Clouds $P_{N_{f}}$, Motion Type $M_{type}$, Segmentation Labels $L$, Instance ID $y$}
    \Output{Motion Axis $\Vec{a}$, Motion Origin $\Vec{o}$} 
    \BlankLine
    {$\Vec{a}, \Vec{o} \leftarrow \Vec{0}, \Vec{0}$}\;
    \tcp{Find $OBB$, where $OBB = (\Vec{v_{1}},\Vec{v_{2}},\Vec{v_{3}},\Vec{c},d_{v_{1}},d_{v_{2}},d_{v_{3}})$}
    $OOB \leftarrow$ \texttt{Find\_Oriented\_Bounding\_Box}$(\mathcal{M}, \ y)$ \;
    $A_{hyp} \leftarrow (\Vec{v_{1}},\Vec{v_{2}},\Vec{v_{3}},-\Vec{v_{1}},-\Vec{v_{2}},-\Vec{v_{3}})$\; 
    $O_{hyp} \leftarrow (\Vec{c} \pm 0.5 \ (d_{v_{1}}.\Vec{v_{1}}), \Vec{c} \pm 0.5(d_{v_{2}}.\Vec{v_{2}}),\Vec{c} \pm 0.5(d_{v_{3}}.\Vec{v_{3}}), \Vec{c})$\;
    $min\_dist \leftarrow 0.0$\;  
    \For{each $\Vec{a_{i}}$ in $A_{hyp}$ }{
    \For{each $\Vec{o_{i}}$ in $O_{hyp}$}{
        %Surface $f$, $\epsilon \leftarrow$ Plane\_Fitting($N_i$)\;
        \tcp{transform vertices of $\mathcal{M}$ as per $M_{type}$ \& find best match.}
        \If{$M_{type}$ = "revolute"}
        {
            
            Mesh $\mathcal{M}^{'} \leftarrow$ \texttt{Revolute}($\mathcal{M}$, $\Vec{a_{i}}$, $\Vec{o_{i}}$, y) \tcp{Eq: \ref{eq: revolute_motion}}
        }
        \If{$M_{type}$ = "prismatic"}
        {
            Mesh $\mathcal{M}^{'} \leftarrow$ \texttt{Prismatic}($\mathcal{M}$, $\Vec{a_{i}}$, y) \tcp{Eq: \ref{eq: prismatic_motion}}
        }
        $P_{\mathcal{M}} \leftarrow$ $\mathcal{M}.$vertices\;
        $e \leftarrow \texttt{chamfer\_distance($P_{\mathcal{M}}$,$P_{N_{f}}$)}$\;
        \If{\texttt{e} < $min\_dist$}
        {
            $\Vec{a} \leftarrow \Vec{a_{i}}$;  $\Vec{o} \leftarrow \Vec{o_{i}}$
        }
            
        }
        
    }
    \caption{Find\_Motion\_Parameters()}
    \label{alg:find_motion_parameters}
\end{algorithm}

\section{Additional Results}
We present additional results on PartNet Sapian Dataset \cite{xiang2020sapien}. The results are shown in Fig. \ref{fig:results partnet sapian}. The part to be articulated is highlighted. As can be seen in the figure, our model is able to generalize within the same category of object of PartNet Sapian Dataset. In addition to this, we also show additional results of the generalization capability of our model on ACD dataset \cite{iliash2024s2o} i.e. the diffusion model is trained on PartNet Sapian dataset and tested on ACD dataset for generalization. As can be seen in Fig. \ref{fig:acd_1} and Fig. \ref{fig:acd_2} can generalize to unseen shapes over a different dataset. We also show articulation results on the 3D mesh in the last column.

\newpage
\begin{figure*}
    \includegraphics[height=\textheight]{images/result_1.png}

\caption{Qualititative results of Multi-View Video Generation and 3D motion axis prediction on PartNet Sapian Dataset.}
\label{fig:results partnet sapian}
\end{figure*}

\newpage
\begin{figure*}
    \includegraphics[width=\textwidth]{images/result_2.png}

\caption{Qualititative results of generalization of Multi-view video generation and 3D Motion Axis prediction on ACD dataset \cite{iliash2024s2o}.}
\label{fig:acd_1}
\end{figure*}

\begin{figure*}
    \includegraphics[width=\textwidth]{images/result_3.png}

\caption{Qualititative results of generalization of Multi-view video generation and 3D Motion Axis prediction on ACD dataset \cite{iliash2024s2o}.}
\label{fig:acd_2}
\end{figure*}
